# Supplementary material for: Authorship recognition via fluctuation analysis of network topology and word intermittency
Source: arXiv:1502.01245 source file (2015-02-04)
Supplement: Supplementary file 1 [file SupplementaryInformation.pdf]

# Authorship recognition via fluctuation analysis of network topology and word intermittency (Supplementary Information)

Diego R. Amancio*
*Department of Computer Science*
*Institute of Mathematical and Computer Sciences*
*University of São Paulo, São Carlos, São Paulo, Brazil*

## I. LIST OF STOPWORDS

Below follows a list of stopwords that were disregarded from the analysis in the pre-processing step.

I A ABOARD ABOUT ABOVE ACROSS AFTER AFTERWARDS AGAINST AGO AGREED-UPON AH ALAS ALBEIT ALL ALL-OVER ALMOST ALONG ALONGSIDE ALTHO ALTHOUGH AMID AMIDST AMONG AMONGST AN AND ANOTHER ANY ANYONE ANYTHING AROUND AS ASIDE ASTRIDE AT ATOP AVEC AWAY BACK BE BECAUSE BEFORE BEFOREHAND BEHIND BEHYNDE BELOW BENEATH BESIDE BESIDES BETWEEN BEWTEEN BEYOND BI BOTH BUT BY CA. DE DES DESPITE DO DOWN DUE DURIN' DURING EACH EH EITHER EN EVERY EVER EVERYONE EVERYTHING EXCEPT FOR FROM GO GODDAMN GOODY GOSH HALF HAVE HE HELL HER HERSELF HEY HIM HIMSELF HIS HO HOW HOWEVER IF IN INSIDE INSOFAR INSTEAD INTO IT ITS ITSELF LA LE LES LEST LIEU LIKE ME MINUS MOREOVER MY MYSELF NEAR NEAR-BY NEARER NEAREST NEITHER NEVERTHELESS NEXT NO NOR NOT NOTHING NOTWITHSTANDING O OER OF OFF ON ONCE ONE ONESELF ONLY ONTO OR OTHER OTHERS OTHERWISE OUR OURS OURSELVES OUT OUTSIDE OUTTA OVER PER RATHER REGARDLESS ROUND SE SHE SHOULD SINCE SO SOME SOMEONE SOMETHING THAN THAT THE THEIR THEM THEMSELVES THEN THERE THEREFORE THESE THEY THINE THIS THOSE THOU THOUGH THROUGH THROUGHOUT THRU TILL TO TOGETHER TOWARD TOWARDS UH UNDER UNDERNEATH UNLESS UNLIKE UNTIL UNTO UP UPON US VIA VIS-A-VIS VIS-'a-VIS WE WELL WHAT WHATEVER WHATSOEVER WHEN WHENEVER WHERE WHEREAS WHEREFORE WHEREUPON WHETHER WHICH WHICHEVER WHILE WHO WHOEVER WHOM WHOSE WHY WITH WITHAL WITHIN WITHOUT YE YEA YEAH YES YET YONDER YOU YOUR YOURS YOURSELF YOURSELVES

* Corresponding author: diego@icmc.usp.br

**Table** S1. List of books employed in the experiments. For each author, five books have been selected.

| **Year** | **Author** | **Title** |
|---|---|---|
| 1892 | Arthur Conan Doyle | The Adventures of Sherlock Holmes |
| 1906 | Arthur Conan Doyle | Through the Magic Door |
| 1898 | Arthur Conan Doyle | The Tragedy of the Korosko |
| 1914 | Arthur Conan Doyle | The Valley of Fear |
| 1900 | Arthur Conan Doyle | The War in South Africa |
| 1903 | Bram Stoker | The Jewel of Seven Stars |
| 1905 | Bram Stoker | The Man |
| 1909 | Bram Stoker | The Lady of the Shroud |
| 1911 | Bram Stoker | The Lair of the White Worm |
| 1914 | Bram Stoker | Dracula's Guest |
| 1842 | Charles Darwin | The Structure and Distribution of Coral Reefs |
| 1844 | Charles Darwin | Geological Observations on the Volcanic Islands |
| 1846 | Charles Darwin | Geological Observations on South America |
| 1872 | Charles Darwin | The Expression of the Emotions in Man and Animals |
| 1877 | Charles Darwin | The Different Forms of Flowers on Plants of the Same Species |
| 1911 | Hector Hugh Munro | Chronicles of Clovis |
| 1912 | Hector Hugh Munro | The Unbearable Bassington |
| 1914 | Hector Hugh Munro | Beasts and Super-Beasts |
| 1913 | Hector Hugh Munro | When William Came |
| 1919 | Hector Hugh Munro | The Toys of Peace |
| 1837 | Charles Dickens | Oliver Twist |
| 1849 | Charles Dickens | David Copperfield |
| 1854 | Charles Dickens | Hard Times |
| 1859 | Charles Dickens | A Tale of Two Cities |
| 1861 | Charles Dickens | Great Expectations |
| 1846 | Herman Melville | Typee: A Peep at Polynesian Life |
| 1847 | Herman Melville | Omoo: A Narrative of Adventures in the South Seas |
| 1851 | Herman Melville | Moby-Dick; or, The Whale |
| 1852 | Herman Melville | Pierre; or, The Ambiguities |
| 1857 | Herman Melville | The Confidence-Man: His Masquerade |
| 1856 | Wilkie Collins | After Dark |
| 1858 | Wilkie Collins | The Woman in White |
| 1862 | Wilkie Collins | No Name |
| 1866 | Wilkie Collins | Armadale |
| 1868 | Wilkie Collins | The Moonstone |
| 1869 | Mark Twain | The Innocents Abroad, or The New Pilgrims' Progress |
| 1872 | Mark Twain | Roughing It |
| 1883 | Mark Twain | Life on the Mississippi |
| 1884 | Mark Twain | Adventures of Huckleberry Finn |
| 1889 | Mark Twain | A Connecticut Yankee in King Arthur's Court |
